# Supplementary material for: Sparse Support Recovery with Non-smooth Loss Functions
Source: arXiv:1611.01030 source file (2016-11-03)
Supplement: Supplementary file 1 [file supplementary.tex]

\documentclass{article}

% if you need to pass options to natbib, use, e.g.:
% \PassOptionsToPackage{numbers, compress}{natbib}
% before loading nips_2016
%
% to avoid loading the natbib package, add option nonatbib:
% \usepackage[nonatbib]{nips_2016}

\usepackage[final]{../nips_2016} % 

% to compile a camera-ready version, add the [final] option, e.g.:
% \usepackage[final]{nips_2016}

\usepackage[utf8]{inputenc} % allow utf-8 input
\usepackage[T1]{fontenc}    % use 8-bit T1 fonts
\usepackage{hyperref}       % hyperlinks
\usepackage{url}            % simple URL typesetting
\usepackage{booktabs}       % professional-quality tables
\usepackage{amsfonts}       % blackboard math symbols
\usepackage{nicefrac}       % compact symbols for 1/2, etc.
\usepackage{microtype}      % microtypography

\usepackage{../mystyle,amssymb,dsfont,amsmath,amsthm,mathtools}

% Some macros to improve readability
\input{../specific-macros.tex}

\title{Sparse Support Recovery with\\Non-smooth Loss Functions:\\
Supplementary Material}

% The \author macro works with any number of authors. There are two
% commands used to separate the names and addresses of multiple
% authors: \And and \AND.
%
% Using \And between authors leaves it to LaTeX to determine where to
% break the lines. Using \AND forces a line break at that point. So,
% if LaTeX puts 3 of 4 authors names on the first line, and the last
% on the second line, try using \AND instead of \And before the third
% author name.

\author{
  Kévin Degraux\\%\thanks{www.uclouvain.be/kevin.degraux} \\
  ISPGroup/ICTEAM, FNRS\\
  Universit\'{e} catholique de Louvain\\
  Louvain-la-Neuve, Belgium 1348 \\
  \texttt{kevin.degraux@uclouvain.be} \\
  %% examples of more authors
  \And
  Gabriel Peyr\'{e}\\%\thanks{gpeyre.github.io/} \\
  CNRS, DMA \\
  \'Ecole Normale Sup\'erieure \\
  Paris, France 75775\\
  \texttt{gabriel.peyre@ens.fr} \\
  \AND
  Jalal M.~Fadili \\
  Normandie Univ, ENSICAEN, \\
  CNRS, GREYC,\\
  Caen, France 14050\\
  \texttt{Jalal.Fadili@ensicaen.fr} \\
  \And
  Laurent Jacques\\% \thanks{perso.uclouvain.be/laurent.jacques/} \\
  ISPGroup/ICTEAM, FNRS\\
  Universit\'{e} catholique de Louvain\\
  Louvain-la-Neuve, Belgium 1348 \\
  \texttt{laurent.jacques@uclouvain.be} \
  %% \And
  %% Coauthor \\
  %% Affiliation \\
  %% Address \\
  %% \texttt{email} \\
}

\begin{document}
% \nipsfinalcopy is no longer used

\maketitle

%%%%%
\input{supplementary-proof.tex}

%\subsubsection*{Acknowledgments}

%To be included in the final paper (on the 9th page).
% \input{acknowledgements.tex}

\small
\bibliographystyle{plain}
\bibliography{library}

\end{document}
